# Supplementary material for: Clustering Based on Graph of Density Topology
Source: arXiv:2009.11612 source file (2020-09-24)
Supplement: Supplementary file 1 [file appendix.tex]

% \documentclass[journal,11pt,draftclsnofoot,twocolumn]{IEEEtran}
% \documentclass{article}
% \usepackage{geometry}
% \usepackage[utf8]{inputenc} % allow utf-8 input
% \usepackage[T1]{fontenc}    % use 8-bit T1 fonts
% \usepackage{hyperref}       % hyperlinks
% \usepackage{url}            % simple URL typesetting
% \usepackage{booktabs}       % professional-quality tables
% \usepackage{amsfonts}       % blackboard math symbols
% \usepackage{nicefrac}       % compact symbols for 1/2, etc.
% \usepackage{microtype}      % microtypography
% \usepackage{lipsum}
% \usepackage{graphicx}
% \graphicspath{ {./images/} }
% \usepackage{caption}
% \usepackage{subfigure}
% \usepackage{amsmath}
% \usepackage{multirow}
% \usepackage{array}
% \usepackage{mathtools}
% \usepackage{bbm}
% \usepackage{algorithm}
% \usepackage{algpseudocode}
% \geometry{a4paper,scale=0.8}

% \usepackage{natbib}  % DO NOT CHANGE THIS AND DO NOT ADD ANY OPTIONS TO IT
% \usepackage{caption} % DO NOT CHANGE THIS AND DO NOT ADD ANY OPTIONS TO IT
% \frenchspacing  % DO NOT CHANGE THIS
% \setlength{\pdfpagewidth}{10in}  % DO NOT CHANGE THIS
% \setlength{\pdfpageheight}{11in}  % DO NOT CHANGE THIS
% \usepackage{amsfonts}
% \usepackage{booktabs}
% \usepackage{makecell}
\renewcommand{\algorithmicrequire}{\textbf{Input:}}  % Use Input in the format of Algorithm
\renewcommand{\algorithmicensure}{\textbf{Output:}} % Use Output in the format of Algorithm

%\nocopyright

% \title{Density Growing Based Structure Finding and Clustering}


% \author{
%  Name1 \\
%   School of Engineering\\
%   Westlake University\\
%   address \\
%   \texttt{name@westlake.edu.cn} \\
%   %% examples of more authors
%   \And
%     Name2 \\
%   School of Engineering\\
%   Westlake University\\
%   address \\
%   \texttt{name@westlake.edu.cn} \\
%   \And
%     Name3 \\
%   School of Engineering\\
%   Westlake University\\
%   address \\
%   \texttt{name@westlake.edu.cn} \\

% }
